# Supplementary material for: Rational boundary charge in one-dimensional systems with interaction and disorder
Source: arXiv:2004.00463 ancillary file (2020-04-01)
Supplement: Supplementary file 1 [file supplemental_material.pdf]

# Supplemental Material: Rational boundary charge in one-dimensional systems with interaction and disorder

Mikhail Pletyukhov,[1] Dante M. Kennes,[1,2] Kiryl Piasotski,[1] Jelena Klinovaja,[3] Daniel Loss,[3] and Herbert Schoeller[1,*]

[1]*Institut für Theorie der Statistischen Physik, RWTH Aachen, 52056 Aachen, Germany and JARA - Fundamentals of Future Information Technology*

[2]*Max Planck Institute for the Structure and Dynamics of Matter, Center for Free Electron Laser Science, 22761 Hamburg, Germany*

[3]*Department of Physics, University of Basel, Klingelbergstrasse 82, CH-4056 Basel, Switzerland*

(Dated: April 1, 2020)

This supplement provides the analysis of the fundamental transformation laws of the boundary charge under translations and local inversion via the relation to the Zak-Berry phase (which is only possible for the special case of noninteracting and clean systems).

## I. BOUNDARY CHARGE AND ZAK-BERRY PHASE

For the special case of noninteracting and clean systems, the boundary charge $Q_B^R \equiv Q_{B,0}^R$ can be related to the Zak-Berry phase $\gamma_R \equiv \gamma_{R,0}$ according to[1–3]

$$Q_B^R = -\frac{\gamma_R}{2\pi} \mod(1). \tag{1}$$

The Zak-Berry phase is defined with respect to the Bloch eigenstates of the bulk Hamiltonian which can be written as

$$\underline{\psi}_k^{(\alpha)}(m) = \frac{1}{\sqrt{2\pi}} \underline{u}_k^{(\alpha)}(m) e^{ikm}, \tag{2}$$

where $-\frac{\pi}{Z} < k < \frac{\pi}{Z}$ defines the 1. Brioullin zone, $\alpha = 1, \ldots, N_c Z$ is the band index, and $\underline{u}_k^{(\alpha)}(m) = \underline{u}_k^{(\alpha)}(m+Z)$ are periodic vector-functions forming a complete, orthogonalized and normalized set of states within the unit cell space for each given quasimomentum $k$

$$\langle \underline{u}_k^{(\alpha)} | \underline{u}_k^{(\alpha')} \rangle = \delta_{\alpha\alpha'} \quad , \quad \sum_\alpha |\underline{u}_k^{(\alpha)}\rangle\langle \underline{u}_k^{(\alpha)}| = \mathbb{1}, \tag{3}$$

with $\langle \underline{u} | \underline{u}' \rangle \equiv \sum_{m=1}^Z \underline{u}^\dagger(m) \underline{u}'(m)$. Conventionally, one chooses the periodic gauge $\underline{\psi}_k^{(\alpha)} = \underline{\psi}_{k+\frac{2\pi}{Z}}^{(\alpha)}$ such that only a phase factor $e^{i\varphi_k^{(\alpha)}}$ with

$$\varphi_k^{(\alpha)} = \varphi_{k+\frac{2\pi}{Z}}^{(\alpha)} \mod(2\pi) \tag{4}$$

leaves a gauge freedom to the Bloch states. As a consequence, the Zak-Berry phase $\gamma_R^{(\alpha)} \equiv \gamma_{R,0}^{(\alpha)}$ for a single band, defined by

$$\gamma_R^{(\alpha)} = i \int_{-\pi/Z}^{\pi/Z} dk \, \langle \underline{u}_k^{(\alpha)} | \partial_k \underline{u}_k^{(\alpha)} \rangle + 2\pi P_{\text{ion}}, \tag{5}$$

is undetermined up to multiples of $2\pi$. The last term is the contribution from the polarization of the ions per band and per unit cell defined by

$$P_{\text{ion}} = -\frac{1}{Z} \sum_{m=1}^{Z} \frac{m}{Z} = -\frac{1+Z}{2Z}, \tag{6}$$

which is again undetermined up to $O(1)$ when the point of reference is shifted by multiples of a lattice vector $Z$. The total Zak-Berry phase $\gamma_R$ is defined by the sum over the occupied bands

$$\gamma_R = \sum_{\alpha=1}^{\nu} \gamma_R^{(\alpha)}. \tag{7}$$

The Zak-Berry phase depends in a subtle way on the definition of the unit cell. This is the point where the precise position of the boundary enters. For a *given* boundary of the system, the convention is to start the unit cell with the first site at the boundary. If we take the semi-infinite Hamiltonian $H_R \equiv H_{R,0}$ this gives the same unit cell as for the bulk Hamiltonian $H_{\text{bulk}}$. For $H_{R,n}$ and $H_{L,n}$ different definitions and inversions of the unit cell have to be taken leading to corresponding changes of the Zak-Berry phase denoted by $\gamma_{R,n}^{(\alpha)}$ and $\gamma_{L,n}^{(\alpha)}$ for each band $\alpha$. Eq. (1) then reads

$$Q_{B,n}^R = -\frac{\gamma_{R,n}}{2\pi} \quad \text{mod}(1)\,, \tag{8}$$

$$Q_{B,n}^L = \frac{\gamma_{L,n}}{2\pi} \quad \text{mod}(1)\,. \tag{9}$$

where $\gamma_{R,n}$ and $\gamma_{L,n}$ are the Zak-Berry phases summed over the number of occupied bands

$$\gamma_{R/L,n} = \sum_{\alpha=1}^{\nu} \gamma_{R/L,n}^{(\alpha)}\,. \tag{10}$$

We note that the relative minus sign between the Zak phases for a semi-infinite system with a left or right boundary is a consequence of the convention that the quasimomentum is defined positive when pointing away or towards the boundary, respectively.

To get the relation between $\gamma_{R,n}$ and $\gamma_R$ we consider a translation $m \to m+n$ and get the following change of the Bloch wave (2)

$$\bar{\psi}_k(m) = \frac{1}{\sqrt{2\pi}}\,\underline{\bar{u}}_k^{(\alpha)}(m) e^{ikm}\,, \tag{11}$$

$$\underline{\bar{u}}_k^{(\alpha)}(m) = \underline{u}_k^{(\alpha)}(m+n) e^{ikn}\,. \tag{12}$$

Obviously, the transformed Zak-Berry phase $\gamma_{R,n}^{(\alpha)}$ for $H_{R,n}$ defined via (5) with respect to $\underline{\bar{u}}_k^{(\alpha)}$ is then given by

$$\gamma_{R,n}^{(\alpha)} = \gamma_R^{(\alpha)} - n\frac{2\pi}{Z}\,, \tag{13}$$

which, via (1), (8) and (10), leads to the transformation law of the boundary charge under translations

$$Q_{B,n}^R = Q_B^R + n\bar{\rho} \quad \text{mod}(1)\,. \tag{14}$$

The Zak-Berry phases $\gamma_R$ and $\gamma_L$ are the same since they are defined with respect to the same lattice and the same unit cell. Using (8) and (9) for $n = 0$ this leads directly to the transformation law of the boundary charge under local inversion

$$Q_B^R + Q_B^L = \text{mod}(1)\,. \tag{15}$$

Although this might look very straigthforward and comparable to the effort needed for the proofs based on the NSP presented in the main part of the paper, this is only possible for noninteracting and clean systems and even in this case, the real work is hidden in the proof of the surface charge theorem (1). This involves the detailed consideration of Wannier function representations as in Ref. [2] or using charge pumping arguments for non-cyclic processes as in Ref. [4]. Whatever proof is used for the relation of the Zak-Berry phase to the boundary charge, the underlying principle is always the NSP. Therefore, instead of using the surface charge theorem, we have preferred in this work to proof the central relations (14) and (15) directly from the NSP to show the deep connection to this principle and to include also the case of short-ranged electron-electron interactions and static random disorder.

---

* Email: schoeller@physik.rwth-aachen.de
[1] R.D. King-Smith and D. Vanderbilt, Phys. Rev. B(R) **47**, 1651 (1993).
[2] D. Vanderbilt and R.D. King-Smith, Phys. Rev. B **48**, 4442 (1993).
[3] R. Resta, Ferroelectrics **136**, 51 (1992); *ibid.* Europhys. Lett. **22**, 133 (1993).
[4] G. Ortiz and R.M. Martin, Phys. Rev. B **49**, 14202 (1994).
